# Supplementary material for: NeuralMPS: Non-Lambertian Multispectral Photometric Stereo via Spectral Reflectance Decomposition
Source: arXiv:2211.15311 source file (2022-11-28)
Supplement: Supplementary file 1 [file supp.pdf]

# NeuralMPS: Non-Lambertian Multispectral Photometric Stereo via Spectral Reflectance Decomposition (Supplementary Material)

Anonymous CVPR submission

Paper ID 3927

## 1. Dynamic shape recovery

Recall that a single input multispectral image (MSI) for multispectral photometric stereo (MPS) encodes observations under varying lighting directions in different spectral bands. Given MSIs captured by a multispectral camera at different timestamps, the proposed MPS method can recover the surface normal of dynamic objects. Please find the attached video for the dynamic shape recovery results of the proposed method. The input MSI sequence records moving hands captured with spectral light sources, which roughly follows the assumptions of the proposed SRD model. As shown in the attached video, the 3D shape of the moving hands in the MSI sequence containing hundreds of frames can be stably reconstructed by the proposed method.

## 2. Code, model and data for evaluation

The code, pretrained model and data for evaluation are available at https://anonymous.4open.science/r/NeuralMPS-689D. Please refer to README.md for configuration and running instructions.

## 3. Effectiveness of the proposed ELIE-Net

We compare the equivalent light intensity estimation results of the proposed ELIE-Net and GO21 [2] on the Sphere and Bunny test dataset. To evaluate the accuracy on the predicted equivalent light intensity, we use "ratio" defined as follows:

$$\text{ratio} = \frac{|e - e_{gt}|}{\max\{e_{gt}, 10^{-3}\}}, \tag{1}$$

where $e$, $e_{gt}$ denote the predicted equivalent light intensity and ground truth, respectively. The results in Fig. 1 demonstrate the superior performance of the proposed ELIE-Net over GO21 [2]. Mean ratios listed in Table 1 show that the proposed ELIE-Net can predict equivalent light intensity nearly 6 times more accurate than GO21 [2].

Table 1: Quantitative results of the predicted equivalent light intensity, which are measured by the mean ratio over 51 materials of the test dataset. Value the lower the better.

| Method | Sphere | Bunny |
|---|---|---|
| Ours | 0.24 | 0.27 |
| GO21 [2] | 1.23 | 1.22 |

## 4. Evaluation on synthetic data

We compare shape recovery results of the proposed method and GO21 on two synthetic examples in Fig. 2. The estimated normal maps and their corresponding error maps and mean angular error (MAE) values are shown. Two representative materials, "ilm_l3_37_metallic" and "ilm_solo_millennium_falcon", are chosen for synthesis. The rendered images of a ball with the chosen materials under different lighting conditions are shown in the last row. As we can see, there are specular reflection on the ball rendered with the first material. While the performance of GO21 [2] varies on these two materials, the proposed method exhibits strong robustness to specular reflection.

## 5. Materials

We select 51 materials from [1] in the paper, whose indices are listed in Table 2.

## References

[1] Jonathan Dupuy and Wenzel Jakob. An adaptive parameterization for efficient material acquisition and rendering. *ACM Trans. on Graph.*, 37(6):1–14, 2018. 1, 2

[2] Heng Guo, Fumio Okura, Boxin Shi, Takuya Funatomi, Yasuhiro Mukaigawa, and Yasuyuki Matsushita. Multispectral photometric stereo for spatially-varying spectral reflectances: A well posed problem? In *Proc. of IEEE Conference on Computer Vision and Pattern Recognition (CVPR)*, pages 963–971, 2021. 1, 2

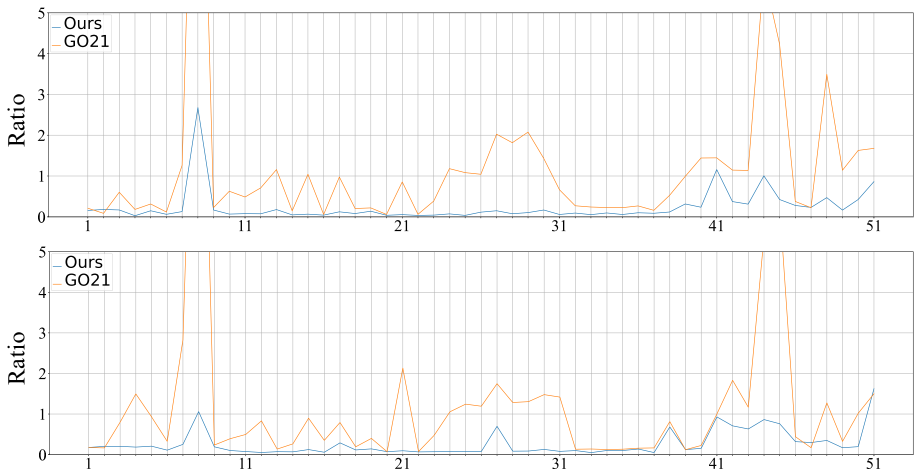


Figure 1: Results of the predicted equivalent light intensity for diverse materials [1] on SPHERE (upper part) and BUNNY (lower part) test dataset. The $X$-axis indicates indices of the materials. The predicted equivalent light intensities are evaluated using "ratio" defined in Eq. (1).

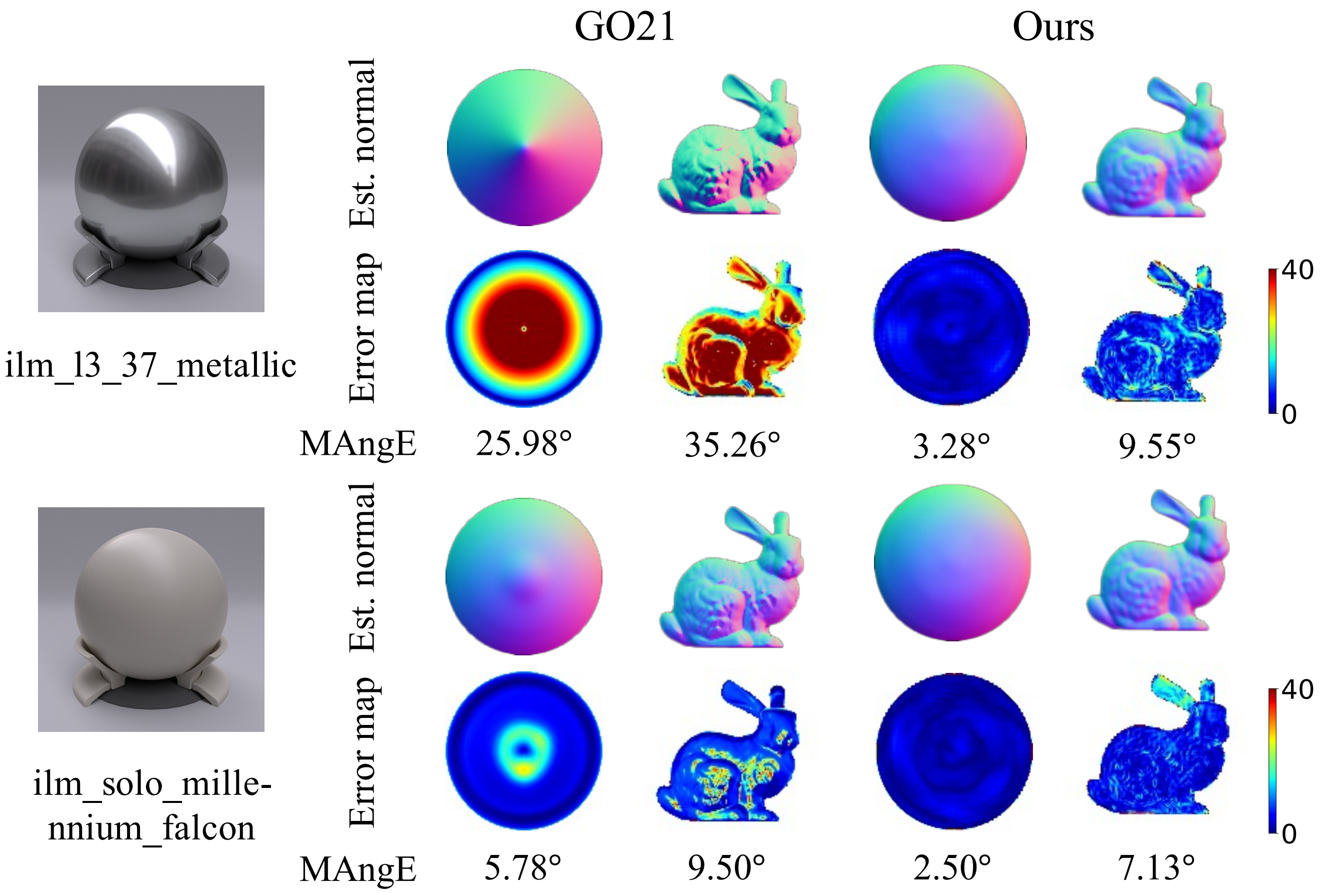


Figure 2: Comparisons of shape recovery results on objects SPHERE and BUNNY rendered with two chosen materials. From top to bottom, the estimated normal maps, their corresponding error maps and mean angular error (MAE) values of the proposed method and GO21 [2] are shown. In addition, the rendered images of a ball with the two chosen materials are shown in the last row. As we can see, there are strong specular reflection on the ball rendered with the first material.

Table 2: Names of materials.

| Index | Name | Index | Name | Index | Name |
|---|---|---|---|---|---|
| 1 | ilm_l3_37_dark_green | 18 | aurora_white | 35 | satin_gold |
| 2 | cm_military_green | 19 | laika_ceiling_paint_18_gray | 36 | satin_rosaline |
| 3 | irid_flake_paint1_fine | 20 | spectralon | 37 | satin_white |
| 4 | ilm_l3_37_matte | 21 | acrylic_felt_purple | 38 | cc_green_malachite |
| 5 | irid_flake_paint1 | 22 | paper_white | 39 | cc_blue_agat |
| 6 | ilm_l3_37_metallic | 23 | paper_blue | 40 | cc_nothern_aurora |
| 7 | ilm_solo_millennium_falcon | 24 | paper_green | 41 | chm_orange |
| 8 | leaf_maple | 25 | paper_yellow | 42 | cc_amber_citrine |
| 9 | irid_flake_paint2 | 26 | acrylic_felt_green | 43 | vch_golden_yellow |
| 10 | cm_toxic_green | 27 | vch_ultra_pink | 44 | vch_silk_blue |
| 11 | colodur_azure_4e | 28 | acrylic_felt_orange | 45 | vch_dragon_eye_red |
| 12 | colodur_napoli_4f | 29 | paper_red | 46 | chm_light_blue |
| 13 | cm_white | 30 | acrylic_felt_pink | 47 | cg_sunflower |
| 14 | colodur_connemara_4c | 31 | acrylic_felt_yellow | 48 | vch_frozen_amethyst |
| 15 | cardboard | 32 | satin_blue | 49 | cc_ibiza_sunset |
| 16 | colodur_kalahari_2a | 33 | acrylic_felt_white | 50 | cc_iris_purple_gem |
| 17 | ilm_solo_m_68 | 34 | satin_purple | 51 | chm_mint |
